# Supplementary material for: Pay Beliefs and the Amenity-Pay Tradeoff
Source: arXiv:2606.02503 source file (2026-06-30)
Supplement: Supplementary file 1 [file tab3_appendix.tex]

\hline
permanent diff, chosen job&      .06111&      .03611&       .0381&       .0494\\
                    &     (.1359)&     (.1468)&     (.1512)&     (.1532)\\
homeoffice diff, chosen job&        .025&      .01889&     .007143&      .01905\\
                    &     (.1108)&     (.1319)&     (.1446)&     (.1267)\\
shift\_work diff, chosen job&     -.05944&     -.03833&     -.05238&     -.02857\\
                    &     (.1276)&     (.1188)&     (.1199)&     (.1234)\\
flextime diff, chosen job&      .07722&      .03611&      .05952&      .06964\\
                    &     (.1743)&     (.1733)&     (.1825)&     (.1863)\\
traveltime diff, chosen job&      -.1982&       -.227&      -.2952&      -.2711\\
                    &     (.5635)&     (.5381)&     (.6023)&     (.6029)\\
training diff, chosen job&    -.008333&      .01389&     -.06964&    -.006548\\
                    &     (.2356)&     (.2098)&     (.2331)&     (.2145)\\
goodcolleagues diff, chosen job&      .02111&      .02611&      .02976&      .01905\\
                    &     (.2039)&     (.1998)&     (.2126)&     (.1936)\\
central diff, chosen job&     .007778&    -.009444&    -.007143&    -.008333\\
                    &     (.2131)&     (.2108)&     (.2171)&     (.2195)\\
otherminorperks diff, chosen job&    .0005556&    -.003333&    -.002381&    -.002381\\
                    &     (.1376)&     (.1148)&     (.1327)&     (.1388)\\
\hline
$                   &         180&         180&         168&         168\\
