# Supplementary material for: Pay Beliefs and the Amenity-Pay Tradeoff
Source: arXiv:2606.02503 source file (2026-06-30)
Supplement: Supplementary file 2 [file tab5_appendix.tex]

\hline
Permanent job           &      0.0979\sym{***}&      0.0447\sym{***}&      0.0332\sym{*}  \\
                    &    (0.0123)         &    (0.0169)         &    (0.0170)         \\
Work from Home &       0.108\sym{***}&      0.0275\sym{*}  &     0.00956         \\
                    &    (0.0153)         &    (0.0160)         &    (0.0162)         \\
Shift Work        &     -0.0816\sym{***}&     -0.0320\sym{*}  &     -0.0243         \\
                    &    (0.0144)         &    (0.0192)         &    (0.0192)         \\
Flexible Hours&    -0.00130         &      0.0157         &      0.0423\sym{**} \\
                    &    (0.0155)         &    (0.0155)         &    (0.0168)         \\
\hline
Number of Observations        &        5,017         &        1,234         &        1,234         \\
Occupation \& Sector Controls     &                     &                     &         Yes         \\
