# Supplementary material for: Pay Beliefs and the Amenity-Pay Tradeoff
Source: arXiv:2606.02503 source file (2026-06-30)
Supplement: Supplementary file 3 [file tab6_appendix.tex]

\hline
Permanent           &       0.210         &       0.109\sym{***}&      0.0767\sym{***}&      0.0768\sym{**} &       0.180\sym{***}\\
                    &                  &   (0.00652)         &   (0.00948)         &    (0.0327)         &    (0.0164)         \\
Home office         &      0.0807         &      0.0789\sym{***}&      0.0439\sym{***}&     0.00111         &      0.0995\sym{***}\\
                    &                  &   (0.00710)         &   (0.00669)         &    (0.0394)         &    (0.0112)         \\
Shift work          &      -0.138         &      -0.181\sym{***}&      0.0193\sym{*}  &      -0.136\sym{***}&      -0.106\sym{***}\\
                    &                  &   (0.00876)         &    (0.0105)         &    (0.0442)         &    (0.0198)         \\
Flexible hours      &      0.0678         &      0.0735\sym{***}&      0.0477\sym{***}&      0.0475         &      0.0756\sym{***}\\
                    &                  &   (0.00700)         &   (0.00615)         &    (0.0311)         &    (0.0104)         \\
Travel time         &     -0.0510         &      -0.130\sym{***}&      -0.147\sym{***}&     -0.0212\sym{**} &      -0.109\sym{***}\\
                    &                  &   (0.00722)         &   (0.00507)         &   (0.00883)         &   (0.00734)         \\
On-the-job Training &                     &                     &                     &     -0.0174         &     -0.0196         \\
                    &                     &                     &                     &    (0.0243)         &    (0.0241)         \\
Good colleagues     &                     &                     &                     &      0.0474\sym{*}  &      0.0396         \\
                    &                     &                     &                     &    (0.0272)         &    (0.0263)         \\
Central location    &                     &                     &                     &      0.0148         &    -0.00680         \\
                    &                     &                     &                     &    (0.0241)         &    (0.0217)         \\
Other minor perks   &                     &                     &                     &    -0.00479         &     -0.0167         \\
                    &                     &                     &                     &    (0.0461)         &    (0.0430)         \\
\hline
Observations        &           .         &         305         &        6960         &        1800         &        8760         \\
Individuals         &                     &                     &         348         &         180         &         348         \\
