# Supplementary material for: Pay Beliefs and the Amenity-Pay Tradeoff
Source: arXiv:2606.02503 source file (2026-06-30)
Supplement: Supplementary file 4 [file tab7A_appendix.tex]

\hline
actual              &     -0.0117         &    -0.00595         &      0.0309\sym{**} &    -0.00758         &     -0.0730         &     0.00179         &    -0.00206         &     -0.0161         &    -0.00294         \\
                    &    (0.0156)         &    (0.0128)         &    (0.0135)         &    (0.0194)         &    (0.0628)         &    (0.0242)         &    (0.0213)         &    (0.0233)         &    (0.0149)         \\
predicted           &     0.00596         &     0.00673         &     -0.0139\sym{**} &      0.0106\sym{*}  &                     &     0.00627         &    -0.00942         &      0.0124         &   -0.000634         \\
                    &   (0.00652)         &   (0.00581)         &   (0.00628)         &   (0.00558)         &                     &   (0.00837)         &   (0.00842)         &   (0.00850)         &   (0.00568)         \\
difference          &     -0.0177         &     -0.0127         &      0.0447\sym{***}&     -0.0181         &                     &    -0.00449         &     0.00736         &     -0.0285         &    -0.00230         \\
                    &    (0.0169)         &    (0.0140)         &    (0.0148)         &    (0.0202)         &                     &    (0.0255)         &    (0.0229)         &    (0.0248)         &    (0.0159)         \\
value\_litt          &    -0.00243         &   -0.000480         &    -0.00425\sym{**} &   -0.000448         &     0.00372         &                     &                     &                     &                     \\
                    &   (0.00324)         &   (0.00103)         &   (0.00185)         &   (0.00115)         &   (0.00320)         &                     &                     &                     &                     \\
value\_subjective    &    -0.00128         &   -0.000470         &    -0.00559\sym{**} &   -0.000557         &     0.00946         &                     &                     &                     &                     \\
                    &   (0.00170)         &   (0.00101)         &   (0.00244)         &   (0.00143)         &   (0.00813)         &                     &                     &                     &                     \\
value\_HCE           &    -0.00210         &   -0.000592         &    -0.00327\sym{**} &   -0.000573         &     0.00798         &  -0.0000351         &  -0.0000816         &    0.000110         &   0.0000491         \\
                    &   (0.00280)         &   (0.00127)         &   (0.00143)         &   (0.00147)         &   (0.00686)         &  (0.000475)         &  (0.000844)         &  (0.000158)         &  (0.000249)         \\
\hline
$ individuals       &         348         &         348         &         348         &         348         &         348         &         348         &         348         &         348         &         348         \\
$ ads               &        1234         &        1234         &        1234         &        1234         &                     &        1234         &        1234         &        1234         &        1234         \\
