# Supplementary material for: Pay Beliefs and the Amenity-Pay Tradeoff
Source: arXiv:2606.02503 source file (2026-06-30)
Supplement: Supplementary file 5 [file willingness_to_pay_appendix.tex]

\hline
Permanent           &       0.158\sym{***}&       0.134\sym{***}&       1.304\sym{***}&      0.0631\sym{***}\\
                    &    (0.0117)         &    (0.0171)         &     (0.367)         &    (0.0138)         \\
Work From Home      &       0.103\sym{***}&     0.00595         &      -0.107         &     -0.0370\sym{*}  \\
                    &   (0.00767)         &    (0.0242)         &     (0.241)         &    (0.0200)         \\
Shift work          &     -0.0825\sym{***}&      -0.105\sym{***}&      -1.751\sym{***}&     -0.0656\sym{***}\\
                    &    (0.0138)         &    (0.0230)         &     (0.522)         &    (0.0190)         \\
Flexible hours      &      0.0691\sym{***}&      0.0791\sym{***}&       1.110\sym{***}&      0.0713\sym{***}\\
                    &   (0.00593)         &    (0.0157)         &     (0.320)         &    (0.0132)         \\
Travel time         &      -0.168\sym{***}&     -0.0305\sym{***}&      -0.358\sym{***}&     -0.0191\sym{***}\\
                    &   (0.00604)         &   (0.00514)         &     (0.108)         &   (0.00377)         \\
\hline
Individuals         &         751         &         704         &         704         &         705         \\
