# Supplementary material for: Pay Beliefs and the Amenity-Pay Tradeoff
Source: arXiv:2606.02503 source file (2026-06-30)
Supplement: Supplementary file 6 [file willingness_to_pay_appendix_slides.tex]

\hline
Permanent           &       0.158\sym{***}&       0.134\sym{***} \\
                    &    (0.0117)         &    (0.0171)                  \\
Work From Home      &       0.103\sym{***}&      0.00595          \\
                    &   (0.00767)         &     (0.0242)  \\
Shift Work          &     -0.0825\sym{***}&      -0.105\sym{***} \\
                    &    (0.0138)         &    (0.0230)                  \\
Flexible Hours      &      0.0691\sym{***}&      0.0791\sym{***} \\
                    &   (0.00593)         &    (0.0157)                  \\
Travel Time         &      -0.168\sym{***}&      -0.0305\sym{***} \\
                    &   (0.00604)         &     (0.00514)                \\
\hline
Individuals         &         751         &         704            \\
